# Supplementary material for: A unified framework for correlation mining in ultra-high dimension
Source: arXiv:2101.04715 source file (2022-08-23)
Supplement: Supplementary file 1 [file redudant_formulae6quantities.tex]

\section{Formulae for \texorpdfstring{$\{N_i^{(k)}: k\in \{\Rma,\Pma\}, i\in \{E_\delta, \breve{V}_\delta, V_\delta \} \}$}{\text{the $6$ quantities}}} 
\label{sec:formulae}

In this section, for $\Psima =\Rma$ or $\Pma$, we write $N_{\VVV_\delta}^{(k)}$, $N_{\VV_\delta}^{(k)}$ and $\Nedged^{(k)}$ in terms of $\Phi_{ij}^{(k)}(\rho)$. The dependence of $\Phi_{ij}^{(k)}(\rho)$ on $\rho$ will be suppressed if it's clear from context.

Define
$$
\breve{C}_i(p-1,l) :=\{\vec{q}: q_1<\dots<q_l, q_{l+1}<\dots<q_{p-1},q_j\in[p]\backslash \{i\},\  q_j\not=q_{j'}, \forall j,j'\in [p-1] \text{ and } j\not = j'\},
$$
and 
$$
C_\delta^{<}:=\{\vec{i}=(i_0,i_1,\cdots,i_\delta)\in [p]^{\delta+1}: i_1<i_2<\cdots<i_\delta, \text{ and } i_l\not= i_0, \forall\ l\in [\delta] \}.
$$

The indicator function when the $i$-the vertex has degree $\delta$ for $1\leq \delta\leq p-1$  is:
$$
\breve{\Phi}_{i,\delta}^{(k)} :=\sum_{\vec{q}\in \breve{C}_i(p-1,\delta)} \prod_{j=1}^\delta \Phi_{iq_j}^{(k)}\prod_{m=\delta+1}^{p-1}(1-\Phi^{(k)}_{iq_m})
$$
The number of vertices with degree $\delta$ for $1\leq \delta\leq p-1$ is:
$$
N_{\VVV_\delta}^{(k)}=\sum\limits_{i=1}^p{\breve{\Phi}_{i,\delta}^{(k)}}
$$

The indicator function when the $i$-the vertex has degree at least $\delta$ for $1\leq \delta\leq p-1$ is:
$$
\Phi_{i,\delta}^{(k)} :=\sum_{l=\delta}^{p-1}\breve{\Phi}_{i,l}^{(k)}
$$
The number of vertices with degree at least $\delta$ for $1\leq \delta\leq p-1$ is:
$$
N_{\VV_\delta}^{(k)}=\sum\limits_{i=1}^p{\Phi_{i,\delta}^{(k)}}
$$

For $1\leq \delta \leq p-1$, define
$$
\mathring{\Phi}_{i,\delta}^{(k)} := \sum_{\vec{q}\in \breve{C}_i(p-1,\delta)}\ \  \prod_{j=1}^\delta \Phi_{iq_j}^{(k)}
= \sum_{\substack{q_1<q_2<\cdots<q_\delta\\q_j\in [p]\backslash \{i\},  \forall j\in [\delta] }}\ \  \prod_{j=1}^\delta \Phi_{iq_j}^{(k)}. $$
$\mathring{\Phi}_{i,\delta}^{(k)}$ is the number of groups of vertices in $[p]\backslash\{i\}$ of size $\delta$ such that the vertex $i$ is connected to each vertex in that group. Thus $\mathring{\Phi}_{i,\delta}^{(k)}=\binom{\text{deg}^{(k)}(i)}{\delta}$, where $\text{deg}^{(k)}(i)$ is the degree of vertex $i$ in empirical correlation graph when $\Psima =\Rma$ or in partial empirical correlation graph when $\Psima =\Pma$. Then for $2\leq \delta \leq p-1$, the number of subgraphs isomorphic to $\Gamma_\delta$ with center at the $i$-th vertex is $\mathring{\Phi}_{i,\delta}^{(k)}$. Thus $\Nedged^{(k)}$ for $1\leq \delta\leq p-1$ is
$$
\Nedged^{(k)}=
\begin{cases}
\sum\limits_{i=1}^p\mathring{\Phi}_{i,\delta}^{(k)} & \text{ when }  2 \leq \delta \leq p-1, \\
2\sum\limits_{1\leq i<j \leq p} \Phi_{ij}^{(k)}= \sum\limits_{i=1}^p\mathring{\Phi}_{i,1}^{(k)} & \text{ when } \delta = 1.
\end{cases} = \sum\limits_{i=1}^p\mathring{\Phi}_{i,\delta}^{(k)} =\sum_{\vec{i}\in C_\delta^<}\ \  \prod_{j=1}^\delta \Phi_{i_0i_j}^{(k)}.
$$
